# Supplementary material for: Visual News: Benchmark and Challenges in News Image Captioning
Source: arXiv:2010.03743 source file (2021-09-13)
Supplement: Supplementary file 1 [file appendix.tex]

\begin{table}[h]
\centering
\small
\begin{tabular}{c|c|c|c|c}
\toprule
 & Guardian & BBC & USA & Wash.\\
\midrule
Number of captions & $602572$ & $198186$ & $151090$ & $128744$ \\
\midrule
% Average Article Length
Number of PERSON\_ & $435629/0.72$ & $92758/0.46$ & $127548/0.84$ & $89811/0.69$ \\
Number of ORG\_ & $225296/0.37$ & $56783/0.29$ & $86276/0.57$ & $55489/0.43$ \\
Number of GPE\_ & $224039/0.37$ & $56897/0.29$ & $78653/0.52$ & $63790/0.50$ \\
Number of DATE\_ & $140325/0.23$ & $43938/0.22$ & $71266/0.47$ & $37528/0.29$ \\
Number of CARDINAL\_ & $77068/0.13$ & $27729/0.14$ & $25992/0.17$ & $11719/0.09$ \\
Number of FAC\_ & $38807/0.06$ & $7628/0.04$ & $23847/0.15$ & $14508/0.11$ \\
Number of NORP\_ & $62865/0.10$ & $19997/0.10$ & $16103/0.11$ & $20124/0.16$ \\
Number of ORDINAL\_ & $22140/0.04$ & $5268/0.03$ & $13177/0.09$ & $4927/0.04$ \\
Number of EVENT\_ & $14215/0.02$ & $2181/0.01$ & $9664/0.06$ & $2928/0.02$ \\
Number of LOC\_ & $24268/0.04$ & $6549/0.03$ & $8907/0.06$ & $6680/0.05$ \\
Number of PRODUCT\_ & $12116/0.02$ & $3259/0.02$ & $5220/0.03$ & $3134/0.02$ \\
Number of TIME\_ & $8664/0.01$ & $3638/0.02$ & $3519/0.02$ & $2755/0.02$ \\
Number of WORK\_OF\_ART\_ & $10593/0.02$ & $1500/0.01$ & $2953/0.02$ & $1810/0.01$ \\
Number of QUANTITY\_ & $4077/0.01$ & $1658/0.01$ & $1414/0.01$ & $957/0.01$ \\
Number of LAW\_ & $1977/0.00$ & $347/0.00$ & $1083/0.01$ & $698/0.01$ \\
Number of MONEY\_ & $1022/0.00$ & $350/0.00$ & $144/0.00$ & $93/0.00$ \\
Number of PERCENT\_ & $81/0.00$ & $17/0.00$ & $64/0.00$ & $184/0.00$ \\
Number of LANGUAGE\_ & $920/0.00$ & $323/0.00$ & $57/0.00$ & $127/0.00$ \\
\bottomrule
\end{tabular}
\caption{Statistics of named entities of four news agencies in \dataset~dataset. For example, the Guardian agency has 602,572 captions and 435,629 PERSON entities, thus each caption will on average have 0.72 PERSON entities. However, each caption only has 0.46 PERSON entities on average in the BBC agency. This difference also demonstrates the diversity of our dataset.}
\label{tab:entities_summary}
\vspace{-0.05in}
\end{table}
